# Supplementary material for: End-to-End Visual Editing with a Generatively Pre-Trained Artist
Source: arXiv:2205.01668 source file (2022-05-03)
Supplement: Supplementary file 1 [file sampling_supp.tex]

\begin{table}[t]
\centering
\scriptsize
\resizebox{0.9\linewidth}{!}{
\begin{tabular}{m{2.8cm}l@{\hskip 0.4in}ll@{\hskip 0.25in}lll@{\hskip 0.15in}c}
\toprule
         &           & \multicolumn{2}{c}{Naturalness (\colorbox{lavenderblue}{$\downarrow$} )}                 & \multicolumn{3}{c}{Faithfulness \colorbox{mistyrose}{($\uparrow$)}}    & Locality (\colorbox{lavenderblue}{$\downarrow$} )    \\ \hline
            % &   & &                & \multicolumn{2}{l}{Inception distribution} & \multicolumn{2}{l}{LPIPS distance}    & \multicolumn{3}{l}{Inception features} & \multicolumn{2}{l}{L1 Outside Edit-Region}                       \\
         &            & Image             & Edit-R                & R@1         & R@5        & R@20        & (L1)                \\ \midrule
% & B: Copy-Paste VQGAN            &   -     &    -        &      \colorbox{mistyrose}{0.974}   &   \colorbox{mistyrose}{0.995}    & \colorbox{mistyrose}{1.000}     &          \colorbox{lavenderblue}{0.049}                        \\
\multirow{3}{*}{\begin{tabular}[c]{@{}l@{}}\textbf{p=1.00}\end{tabular}}  & \textit{Dresses-7m}              &   13.609   & 26.854         & 0.764    & 0.922    & 0.972      & 0.058              \\  
  & FFHQ            &   11.750    & 11.422              &   0.850     & 0.967     & 0.994       & 0.109                                \\  
   & LSUN Bedrooms                 & 13.952 &  24.341           &  0.764    & 0.917     &  0.980    & 0.121                               \\  \midrule
 \multirow{3}{*}{\begin{tabular}[c]{@{}l@{}}\textbf{p=0.98}\end{tabular}}  & \textit{Dresses-7m}              &  13.786    &    25.903      & 0.779   & 0.925    & 0.975      & 0.057              \\  
  & FFHQ            &   11.925    &     11.140         &    0.852    & 0.967    &  0.995     &  0.108                              \\  
   & LSUN Bedrooms                 & 14.084 &  23.513           &  0.772    & 0.918     &   0.982   & 0.121                               \\  \midrule
\multirow{3}{*}{\begin{tabular}[c]{@{}l@{}}\textbf{p=0.96}\end{tabular}}  & \textit{Dresses-7m}              &   13.977   &     25.522     & 0.783    & 0.926   &  0.977    &  0.057             \\  
  & FFHQ            &    12.154   &     10.981         &    0.857    & 0.968     & 0.995      & 0.107                                \\  
   & LSUN Bedrooms                 & 14.021 &  23.193           &   0.773   & 0.914     & 0.982     & 0.120                               \\  \midrule
\multirow{3}{*}{\begin{tabular}[c]{@{}l@{}}\textbf{p=0.94}\end{tabular}}  & \textit{Dresses-7m}              & 14.043      &    25.282       &  0.783     &     0.927  &    0.977    & 0.056                      \\  
  & FFHQ            &  12.394      &        10.841          &   0.852      &    0.967     & 0.993          &        0.107                                   \\  
   & LSUN Bedrooms                 &  14.173      &     22.927            &     0.778     &     0.913    &  0.979       & 0.119                                  \\  \midrule
\multirow{3}{*}{\begin{tabular}[c]{@{}l@{}}\textbf{p=0.92}\end{tabular}}  & \textit{Dresses-7m}              & 14.196      &    25.064       &  0.791     & 0.933      &    0.978    &  0.056                      \\  
  & FFHQ            &    12.506    &    10.642              &   0.854      & 0.966         &    0.994       &  0.106                                         \\  
   & LSUN Bedrooms                 &    14.199    &    22.921             &  0.780         &    0.925     &     0.982    &        0.119                           \\  \midrule
   \multirow{3}{*}{\begin{tabular}[c]{@{}l@{}}\textbf{p=0.9}\end{tabular}}  & \textit{Dresses-7m}              &   14.411    & 24.743          &    0.797  &    0.937   & 0.960       &             0.056          \\  
  & FFHQ            &    12.770    &    10.574              &   0.853      &    0.970     & 0.994          &    0.106                                       \\  
   & LSUN Bedrooms                 &    14.107    &22.187                 & 0.789         &     0.923    & 0.981        &  0.119                                 \\  \midrule
   \multirow{3}{*}{\begin{tabular}[c]{@{}l@{}}\textbf{p=0.88}\end{tabular}}  & \textit{Dresses-7m}              &   14.477    & 24.574          & 0.798     &  0.936      &     0.978   &0.056                       \\  
  & FFHQ            &    13.034    &    10.535              & 0.857        &    0.968     &0.995           &            0.105                               \\  
   & LSUN Bedrooms                 &   14.352     &     21.962            &     0.785     &  0.917        &     0.982    &  0.118                                 \\  \midrule
   \multirow{3}{*}{\begin{tabular}[c]{@{}l@{}}\textbf{p=0.86}\end{tabular}}  & \textit{Dresses-7m}              &   14.610    &     24.315      & 0.798     &  0.936     &  0.977      &    0.056                   \\  
  & FFHQ            &    13.234    &        10.454          &   0.855      &    0.968     & 0.994          &        0.105                                   \\  
   & LSUN Bedrooms                 &   14.540     &     21.984            & 0.785         &  0.920        &     0.982    &          0.118                         \\  \midrule
    \multirow{3}{*}{\begin{tabular}[c]{@{}l@{}}\textbf{p=0.84}\end{tabular}}  & \textit{Dresses-7m}              &   14.609    &    24.164       &   0.799   & 0.936      &     0.979   & 0.056                      \\  
  & FFHQ            &    13.449    &        10.446          &   0.856      &    0.966     & 0.994          &        0.104                                   \\  
   & LSUN Bedrooms                 &   14.630     &     22.216            & 0.792         & 0.915        & 0.982        &               0.118                    \\  \midrule
    \multirow{3}{*}{\begin{tabular}[c]{@{}l@{}}\textbf{p=0.82}\end{tabular}}  & \textit{Dresses-7m}              &   14.774    &    24.193       &  0.800    & 0.936      &  0.977       &      0.055                 \\  
  & FFHQ            &   13.633   & 10.334            &  0.856 &     0.968 &     0.995  &        0.104                              \\  
   & LSUN Bedrooms                 &  14.745      &     22.057            &     0.794     &  0.921        & 0.984        &  0.117                                 \\  \midrule
  \multirow{3}{*}{\begin{tabular}[c]{@{}l@{}}\textbf{p=0.00}\end{tabular}}  & \textit{Dresses-7m}              &    26.610  & 36.402         &  0.645  & 0.837    & 0.933      &0.055               \\  
  & FFHQ            &    29.628   &     27.020         & 0.750        & 0.904    & 0.974      & 0.102                               \\  
   & LSUN Bedrooms                 & 45.267 &  74.458           &   0.652   & 0.840     & 0.953     & 0.116                               \\  \midrule
          \multirow{3}{*}{\begin{tabular}[c]{@{}l@{}}\textbf{k=1}\end{tabular}}  & \textit{Dresses-7m}              &   26.609   & 36.402        & 0.645   & 0.837    & 0.933  &    0.055              \\  
  & FFHQ            &  29.628   &  27.020         &  0.750  & 0.904      & 0.974     & 0.102                              \\  
   & LSUN Bedrooms                 &   45.266     & 75.458               &  0.625       &  0.840       &         0.953 &    0.116                            \\  \midrule
       \multirow{3}{*}{\begin{tabular}[c]{@{}l@{}}\textbf{k=50}\end{tabular}}  & \textit{Dresses-7m}              &   14.262   &    25.320     & 0.800   & 0.936   & 0.981  &  0.057                \\  
  & FFHQ            &  12.456   &  10.445         & 0.858  &    0.972   & 0.995    &    0.108                          \\  
   & LSUN Bedrooms                 &   14.179     &     21.818          &   0.781      &    0.924     &     0.982    & 0.120                               \\  \midrule
          \multirow{3}{*}{\begin{tabular}[c]{@{}l@{}}\textbf{k=100}\end{tabular}}  & \textit{Dresses-7m}              &  13.935    &    25.861     & 0.786   & 0.929    &  0.977 &  0.057                \\  
  & FFHQ            & 12.131    &     10.732      & 0.855  &    0.967  &    0.995 &0.109                              \\  
   & LSUN Bedrooms                 &    14.061    &     22.375          &   0.780      &    0.925     &     0.980    & 0.121                               \\  \midrule
          \multirow{3}{*}{\begin{tabular}[c]{@{}l@{}}\textbf{k=150}\end{tabular}}  & \textit{Dresses-7m}              &   13.766   &    25.984     & 0.775   & 0.927   & 0.976  & 0.057                 \\  
  & FFHQ            &  11.890   &  10.859         & 0.853  &    0.967  &    0.994 &0.109                              \\  
   & LSUN Bedrooms                 &  14.005      &     22.965          &   0.779      &    0.920     & 0.981        & 0.121                               \\  \midrule
          \multirow{3}{*}{\begin{tabular}[c]{@{}l@{}}\textbf{k=200}\end{tabular}}  & \textit{Dresses-7m}              &   13.740   &    26.410     & 0.777  & 0.929    & 0.975  & 0.057                 \\  
  & FFHQ            &  11.807   &  11.094         & 0.851  &    0.970  &0.994     & 0.109                              \\  
   & LSUN Bedrooms                 &  13.994      &     23.508          &  0.771       &    0.922     & 0.981        & 0.121                               \\  \midrule
          \multirow{3}{*}{\begin{tabular}[c]{@{}l@{}}\textbf{k=250}\end{tabular}}  & \textit{Dresses-7m}              &   13.712   &    26.512     & 0.772   & 0.926    & 0.974 & 0.057                 \\  
  & FFHQ            & 11.752    & 11.215          & 0.850   & 0.969     & 0.995    & 0.109                              \\  
   & LSUN Bedrooms                 &    13.961    &         23.579      &   0.773      &    0.918     & 0.980        & 0.121                               \\  \midrule
     \multirow{3}{*}{\begin{tabular}[c]{@{}l@{}}\textbf{k=350}\end{tabular}}  & \textit{Dresses-7m}              &   13.639   & 26.684         & 0.765    & 0.923    & 0.972      & 0.058              \\  
  & FFHQ            &    11.739   &     11.401         &    0.850    & 0.967     &  0.995     & 0.109                                \\  
   & LSUN Bedrooms                 & 14.004 & 24.233            &    0.768  & 0.917     &   0.981   & 0.121                               \\  \midrule
     \multirow{3}{*}{\begin{tabular}[c]{@{}l@{}}\textbf{k=450}\end{tabular}}  & \textit{Dresses-7m}              &  13.612    & 26.849          &  0.764  & 0.922   & 0.972     &   0.058            \\  
  & FFHQ            &   11.744    & 11.428             & 0.850        & 0.967    & 0.994       &    0.109                            \\  
   & LSUN Bedrooms                 & 14.000 &  24.280           & 0.771      & 0.918     & 0.980     & 0.121                               \\  \midrule
     \multirow{3}{*}{\begin{tabular}[c]{@{}l@{}}\textbf{k=550}\end{tabular}}  & \textit{Dresses-7m}              &   13.605   &     26.851     & 0.764    & 0.922   & 0.972     & 0.058              \\  
  & FFHQ            &   11.744    &     11.429         & 0.850        & 0.967    & 0.994       &    0.109                            \\  
   & LSUN Bedrooms                 & 13.940 &  24.287           & 0.764     & 0.916     &  0.981    &  0.121                              \\  \midrule
     \multirow{3}{*}{\begin{tabular}[c]{@{}l@{}}\textbf{k=650}\end{tabular}}  & \textit{Dresses-7m}              &   13.605   & 26.851         & 0.764    & 0.922   & 0.972     &       0.058        \\  
  & FFHQ            &   11.745    & 11.425             &    0.850    & 0.967    &  0.994     &      0.109                          \\  
   & LSUN Bedrooms                 & 13.941 &  24.343           & 0.764     & 0.917     & 0.981     &  0.121                              \\  \midrule
       \multirow{3}{*}{\begin{tabular}[c]{@{}l@{}}\textbf{k=1024}\end{tabular}}  & \textit{Dresses-7m}              &   13.605   & 26.850         & 0.764   & 0.922   & 0.972     & 0.058              \\  
  & FFHQ            &  11.747     & 11.426             & 0.850        & 0.967    & 0.994       &    0.109                            \\  
   & LSUN Bedrooms                 & 13.944 &  24.356            & 0.764     & 0.917      & 0.981     & 0.121                               \\  \midrule
  \bottomrule

\end{tabular}
} 
\vspace{1mm}
\caption{\label{sampling_table}. \footnotesize{ Parameter sweep over the sampling parameters. If I have time then this should be turned into 6 different graphs with the metrics all plotted }}

\end{table}
